# Supplementary material for: A ferroelectric liquid crystal confined in cylindrical nanopores: Reversible smectic layer buckling, enhanced light rotation and extremely fast electro-optically active Goldstone excitations
Source: arXiv:1711.09673 ancillary file (2017-11-27)
Supplement: Supplementary file 1 [file Electronic_Supporting_Information.pdf]

# Electronic Supporting Information

## A ferroelectric liquid crystal confined in cylindrical nanopores: Reversible smectic layer buckling, enhanced light rotation and extremely fast electro-optically active Goldstone excitations


Mark Busch[1], Andriy V. Kityk[1,2,*] Wiktor Piecek[3], Tommy Hofmann[4], Dirk Wallacher[4], Sylwia Całus[2], Przemysław Kula[3], Martin Steinhart[5], Manfred Eich[6,7], and Patrick Huber[1†]

[1] *Institute of Materials Physics and Technology, Hamburg University of Technology, 21073 Hamburg, Germany*
[2] *Faculty of Electrical Engineering, Czestochowa University of Technology, Al. Armii Krajowej 17, 42-200 Czestochowa, Poland*
[3] *Military University of Technology, Kaliskiego Str. 2, 00-908 Warsaw, Poland*
[4] *Helmholtz-Zentrum Berlin für Materialien und Energie GmbH, 14109 Berlin, Germany*
[5] *Institute for the Chemistry of New Materials, University Osnabrück, 49067 Osnabrück, Germany*
[6] *Institute of Optical and Electronic Materials, Hamburg University of Technology, 21073 Hamburg, Germany*
[7] *Institute of Materials Research, Helmholtz-Zentrum Geesthacht, Max-Planck-Straße 1, 21502 Geesthacht, Germany*



(Dated: September 25, 2017)



* E-mail: andriy.kityk@univie.ac.at
† E-mail: patrick.huber@tuhh.de

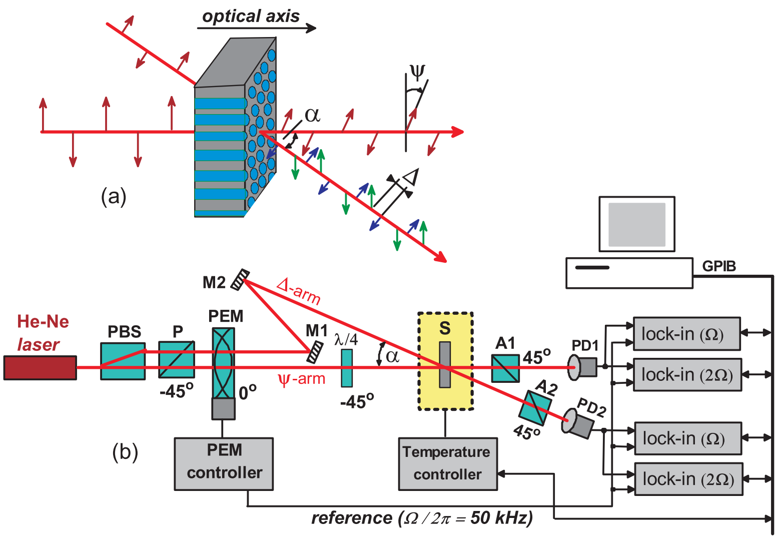


FIG. 1. Illustration of the optical experiments: (a) The FLC-filled mesoporous anodized aluminum oxide (AAO) membrane represents an uniaxial anisotropic medium with the optical axis parallel to the long channel axis of the cylindrical nanochannels. Chiral molecules embedded in the channels result in two types of optical anisotropy: (i) circular birefringence characterized by a rotation of light polarization, $\Psi$, and (ii) linear birefringence leading to an optical retardation, $\Delta$. These characteristics can be probed by polarized light propagating either parallel to the channel axis or under an angle $\alpha$ to it, respectively. (b) Optical polarimetry setup which allows one to simultaneously measure both optical quantities. The key experimental building blocks are a polarization beam splitter (PBS), a polarizer (P), two analyzers (A1 and A2), a photoelastic modulator (PEM), two mirrors (M1 and M2) and a quarter-wave plate ($\lambda/4$). The modulated intensities of light in the $\Psi$- and $\Delta$-arm are detected by the photodiodes PD1 and PD2, respectively, and subsequently analyzed by two pairs of lock-in amplifiers communicating with a PC via GPIB. The angular orientations of optical elements are indicated.

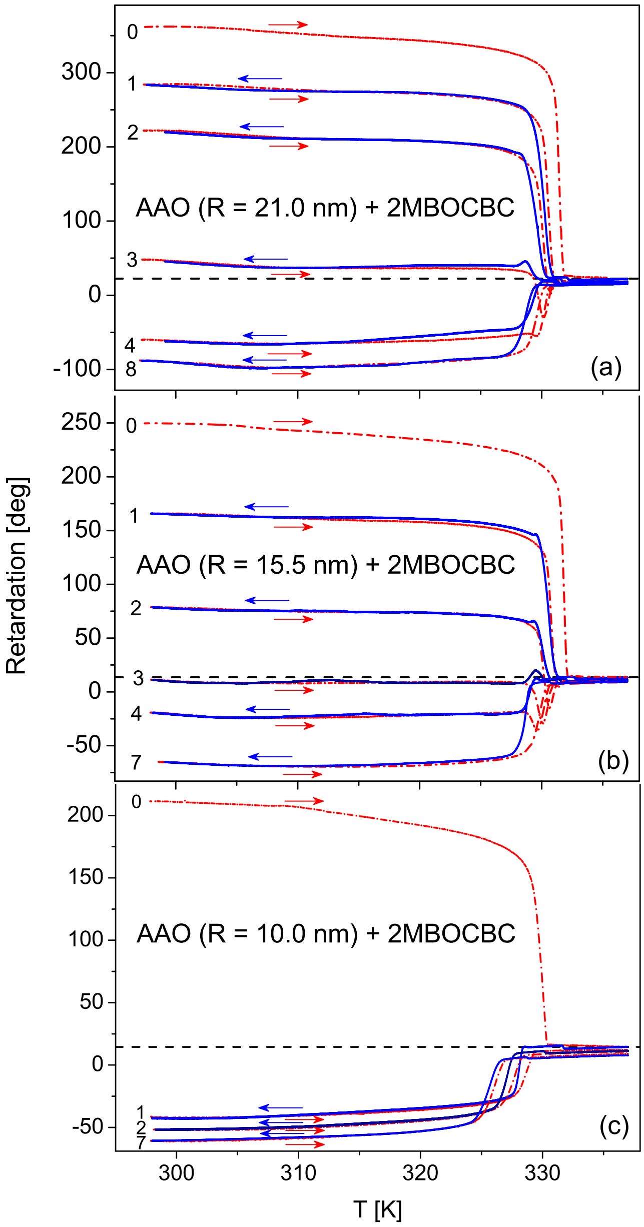


FIG. 2. Temperature dependences of the optical retardation $\Delta$ measured in a sequence of cooling/heating runs (incident angle $\alpha = 36$ deg) in FLC based nanocomposites with untreated AAO membrane of different capillary radii. Panel (a): $R = 21$ nm, panel (b): $R = 15.5$ nm, panel (c): $R = 10$ nm. The number of the cooling/heating run is indicated in the figure. For clarity, not all runs are shown. The initial heating run, performed immediately after the filling of the nanoporous membranes by FLC 2MBOCBC, is labeled with 0. Heating and cooling runs correspond to dash-dot red and solid blue curves, respectively. Initially, the retardation is positive at low temperature, indicating tangential alignment of the FLC. However, the retardation after each heating scan decreases to smaller and smaller values at low $T$. Starting with the 3., 2. and 0. cycle respectively, it turns even negative as a function of decreasing channel diameter, indicating a transformation towards a dominantly radial orientation of the molecules. Thus, the native AAO walls do not provide a temperature-stable tangential alignment of the FLC molecules. We rather observe an irreversible, heating-cooling cycle dependent transformation from tangential (planar wall anchoring) to radial alignments of the FLC mesogens.

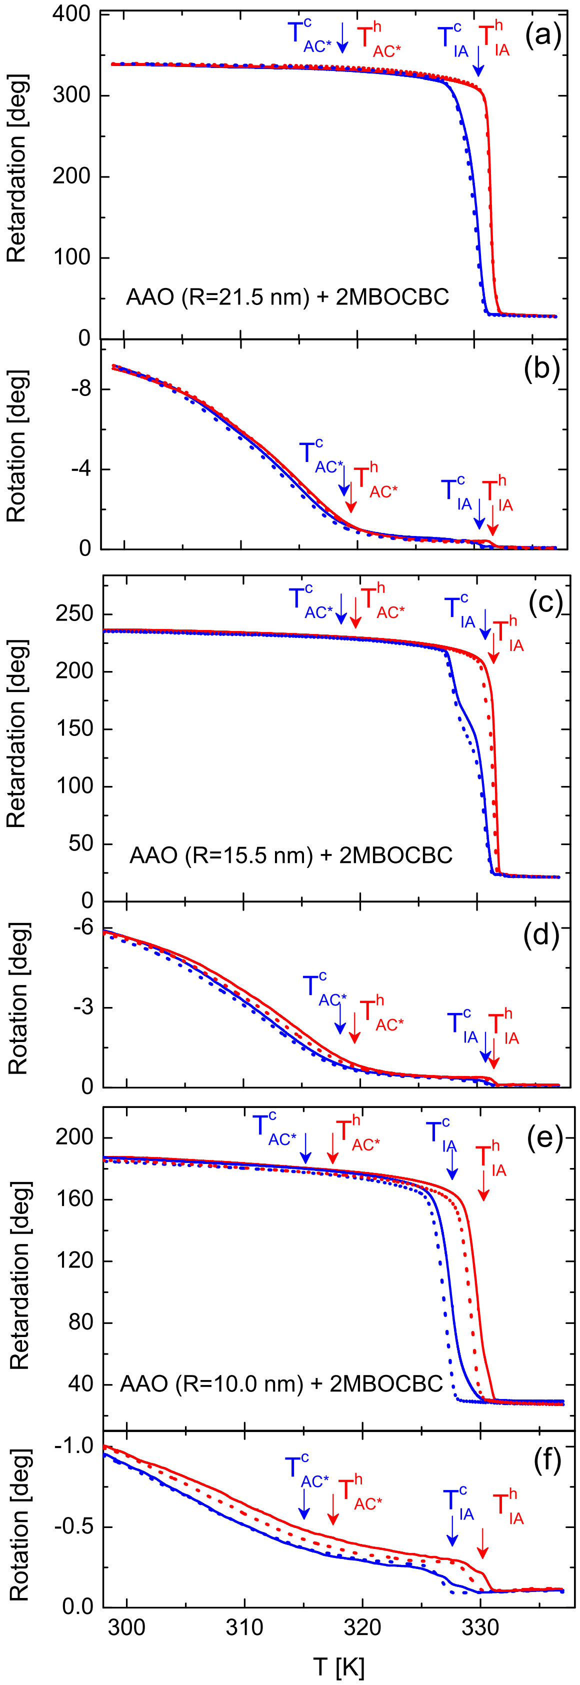


FIG. 3. Temperature dependences of the optical retardation $\Delta$ (incident angle $\alpha = 36$ deg, upper subpanels (a), (c) and (e)) and optical rotation $\Psi$ (lower subpanels (b), (d) and (f)) measured in FLC 2MBOCBC embedded into nanocapillaries of host AAO membranes of different capillary radii (see labels) with capillary walls coated by polymer SE-130. Nanometric capillary walls coating by polymer SE-130 results to a stabilization of the axial molecular arrangement due to enhancing of tangential type anchoring in the interface region; The temperature behavior of both optical activity and optical retardation in subsequent measuring heating/cooling runs is practically recoverable; Only the first (solid curves) and forth (broken curves) heating/cooling runs are shown. The negative sign in the lower subpanels indicates that the rotation direction is lefthanded (counterclockwise).

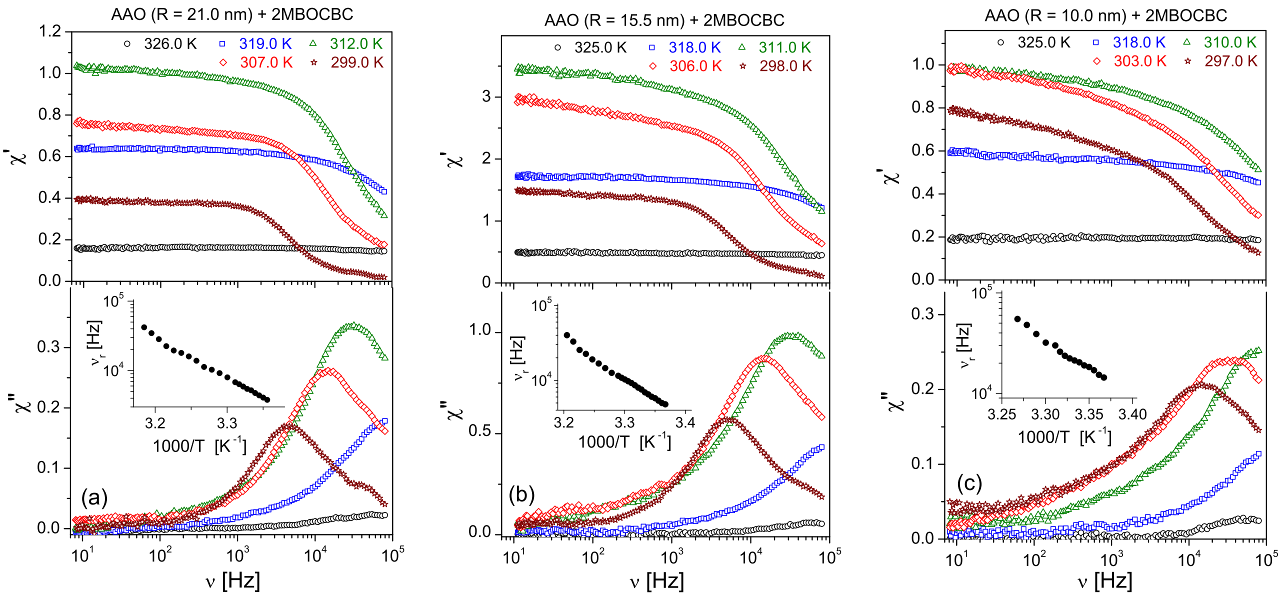


FIG. 4. Real and imaginary parts of the linear electro-optical response, $\chi'$ and $\chi''$ vs frequency $\nu$ of the SmA and SmC* phases confined in polymer coated AAO membranes with different capillary radii for selected temperatures. Insets contain Arrhenius plots for the phason relaxation frequency determined from maxima positions of the $\chi''(\nu)$-dependences.

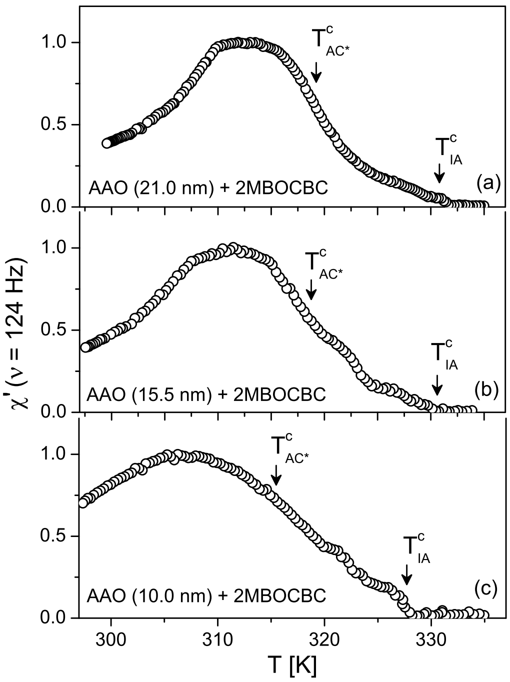


FIG. 5. Real part of the normalized linear electro-optical response, $\chi'$ vs $T$, measured at constant frequency corresponding to quasistatic regime ($\nu = 124$ Hz $\ll \nu_r$) in FLC based nanocomposites with polymer treated AAO matrices of different channel radii, see labeled. The presented dependences are normalized to their maximum value.
